# Supplementary material for: Orbital angular momentum transfer to stably trapped elastic particles in acoustical vortex beams
Source: arXiv:1804.01272 source file (2018-07-05)
Supplement: Supplementary file 1 [file supp_matRevision1.pdf]

# Orbital angular momentum transfer to stably trapped elastic particles in acoustical vortex beams

Diego Baresch and Jean-Louis Thomas

*Sorbonne Université, CNRS UMR 7588,*

*Institut des NanoSciences de Paris, INSP, F-75005, Paris, France.**

Régis Marchiano

*Sorbonne Université, CNRS UMR 7190,*

*Institut Jean le Rond d'Alembert, F-75005, Paris, France.*

## SUPPLEMENTARY MATERIALS

### Rotation rate measurement and control

To measure the rotation rate, we first trap the particle by switching on the AV. The particle is stably held in place for minutes or hours. We record the motion of the janus particle at 159 fps (Fig.1a) and analyze the fluctuations of the mean gray area of the particle (ImageJ, `https://imagej.nih.gov/ij/index.html`) on Fig. 1b. The mean gray area grows with the optic intensity twice in a revolution. This occurs when light is transmitted through the particle and towards the camera. In those moments, the golden layer is not facing directly the light source or the camera. Instead, the mean gray value drops when the golden layer obstructs the light transmission.

The rotation rate can be controlled by switching dynamically the handedness of the AV (see main text). In Fig.1 b, the black curve detects the rotation rate at full anti-clockwise excitation ($m = -1$), while the blue curve is obtained for an anti-clockwise excitation only 75% of the time period $T_0 = 400\mu$s. In Fig1. c we summarize the control of the rate from 0 to ∼11 Hz. Evidently, the rotation direction can be totally inverted.

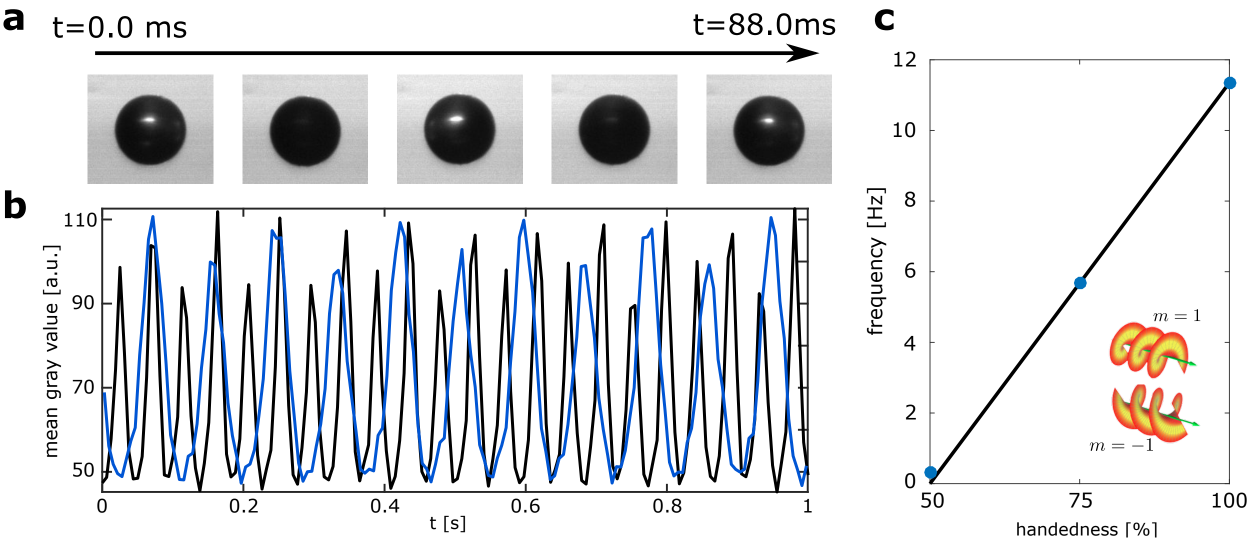


FIG. 1. Rotation rate measurement. a) Time lapse of a spinning and trapped particle. b) Detection of the rotation rate with the mean gray area. c) AV dynamic handedness control in percentage of anticlockwise OAM.

**Rotational streaming flow**

The rotational flow is measured by tracking the optical boundary that becomes visible as ink is injected near the focal zone (Fig2. b in main text). We can follow the evolution in time of the two regions on the propagation axis (at $x = 0$ in Fig2.c main text) when the AV is switched on and after the injection needle is totally removed. Fig2. a shows a color plot of this evolution. Before $t \sim 1.2$ s, the black region (ink) is located near the focal distance ($z < 1$ mm). At $t \sim 1.2$ s the AV is turned on and the flow is initiated, moving the ink downwards. This time evolution $z(t)$ of the ink/water frontier gives us a good estimate of the streaming flow, $u_z(t)$, after interpolation and differentiation (Fig2. b). We can finally plot $u_z(z)$ that is maximum near the focus ($u_z \sim 4.3$ mm/s at $z = 0$). The rotational component (see main text) can be evaluated in the same way and is found to be smaller ($u_\varphi \sim 1$ mm/s).

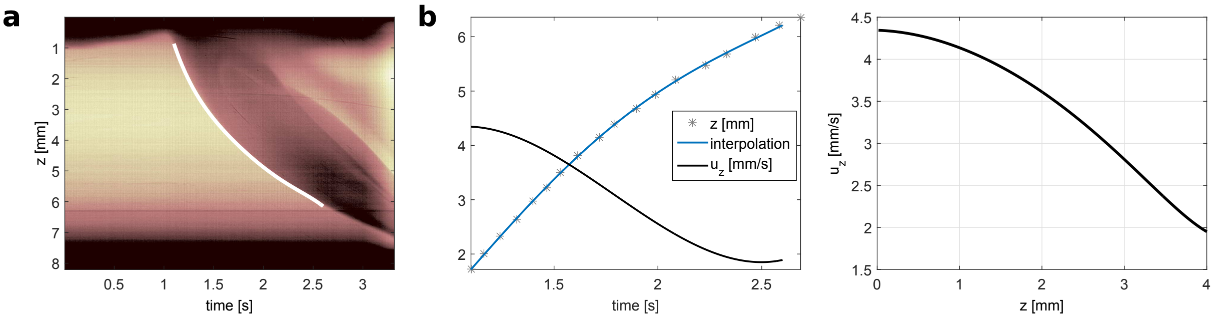


FIG. 2. Streaming flow evaluation. a) Evolution of the ink (dark)/water(bright) frontier as the AV is switched on. b)-c) Calculation of the axial streaming component $u_z$ as a function of $t$ and $z$.

**Acoustic radiation torque exerted on an oscillating visco-elastic sphere in a viscous fluid**

In this section we calculate the acoustic radiation torque exerted by a focused vortex beam on a sphere made of a visco-elastic material in a viscous fluid. Following the notations in Ref.[1], the acoustic radiation torque along $z$ for a sphere *on the axis* for the beam is found to be

$$\Omega_z = \frac{m}{\omega} P_{abs}, \tag{1}$$

in agreement with [2, 3], where

$$P_{abs} = -\frac{2\pi\langle I\rangle}{k^2}\sum_{n=m}^{\infty}\frac{2(n+m)!}{(2n+1)(n-m)!}|A_n^m|^2\left[|R_n|^2 \right.$$
$$\left. + \quad \Re(R_n)\right], \tag{2}$$

is the power absorbed by a sphere located on the axis of a beam having a phase helicity $e^{im\varphi}$, beam shape coefficients $A_n^m$ and mean intensity $\langle I\rangle = p_0^2/(2\rho c)$. The beam shape coefficients $A_n^m$ can be obtained from Ref.[4] for an AV focused by a concave emitter with radius of curvature $r_0 = 6.8$cm and emitter aperture radius $a_0 = 4.5$ cm. Note that the computed beam was shown to be in very good agreement with the experimental field measured with a needle hydrophone [5].

From Eq.(1), it is obvious that the torque will vanish for an axisymmetric beam with $m = 0$. Additionally, for an ideal non-absorptive spherical object placed in an ideal fluid, $P_{abs}$ will vanish. Otherwise, absorption processes in a thermo-viscous fluid for an absorbing sphere are accounted for in the expression of the scattering coefficients $R_n$. The visco-elastic properties of polystyrene, like many amorphous solids with a glass transition, can be well modeled as a Maxwell material. The bulk and shear coefficients are frequency dependent and have been reported in Ref.[6], [7] in the low MHz regime as follows: density $\rho_p = 1050$ kg/m$^3$, longitudinal wave velocity $c_\ell^\infty = 2350$ m/s, transverse wave velocity $c_t^\infty = 1100$ m/s and absorption coefficients $\alpha_\ell = 30$ Np/m and $\alpha_t = 100$ Np/m respectively. Under these conditions, the phase velocity for bulk longitudinal and shear waves are corrected as follows:

$$c_\ell^p(\omega) = c_\ell^\infty/(1 + \mathrm{i}\alpha_\ell c_\ell^\infty/\omega), \tag{3}$$

$$c_t^p(\omega) = c_t^\infty/(1 + \mathrm{i}\alpha_t c_t^\infty/\omega). \tag{4}$$

The later is related to the complex shear modulus:

$$G^p = \rho_p(c_t^\infty)^2/(1 + \mathrm{i}\alpha_t c_t^\infty/\omega)^2. \tag{5}$$

The scattering coefficients $R_n$ can be obtained from the boundary conditions on the particle's surface and reduces to a $4 \times 4$ linear system of differential equations, $\mathbf{A}X = \mathbf{B}$, where:

$$A_{11} = x_\ell h_n'(x_\ell), \tag{6}$$

$$A_{12} = h_n(x_\ell), \tag{7}$$

$$A_{13} = G\left(b_n h_n(x_\ell) - 4x_\ell h_n'(x_\ell)\right), \tag{8}$$

$$A_{14} = G(x_\ell h_n'(x_\ell) - h_n(x_\ell)), \tag{9}$$

$$A_{21} = \frac{1}{2}a_n h_n(x_t), \tag{10}$$

$$A_{22} = x_t h_n'(x_t) + h_n(x_t), \tag{11}$$

$$A_{23} = G a_n(x_t h_n'(x_t) - h_n(x_t)), \tag{12}$$

$$A_{24} = G(c_n h_n(x_t) - x_t h_n'(x_t)), \tag{13}$$

$$A_{31} = -x_\ell^p j_n'(x_\ell^p), \tag{14}$$

$$A_{32} = -j_n(x_\ell^p), \tag{15}$$

$$A_{33} = -G^p(b_n^p j_n(x_\ell^p) - 4x_\ell^p j_n'(x_\ell^p)), \tag{16}$$

$$A_{34} = -G^p(x_\ell^p j_n'(x_\ell^p) - j_n(x_\ell^p)), \tag{17}$$

$$A_{41} = -\frac{1}{2}a_n j_n(x_t^p), \tag{18}$$

$$A_{42} = -(x_t^p j_n'(x_t^p) + j_n(x_t^p)), \tag{19}$$

$$A_{43} = -G^p a_n(x_t^p j_n'(x_t^p) - j_n(x_t^p)), \tag{20}$$

$$A_{44} = -G^p(c_n^p j_n(x_t^p) - x_t^p j_n'(x_t^p)), \tag{21}$$

with $a_n = 2n(n+1)$, $b_n = a_n - (x_t)^2$, $b_n^p = a_n - (x_t^p)^2$, $c_n = b_n/2 - 1$, $c_n^p = b_n^p/2 - 1$, $j_n$ and $h_n$ are spherical bessel and first order hankel functions respectively, $x$ stands for the non-dimensional wave numbers $x = ka = (\omega/c)a$, the superscript $p$ is used to distinguish waves propagating inside the particle. In the liquid, the subscrit $\ell$ and $t$ are used to identify longitudinal and transverse velocity and $G = -i\omega\mu$ where $\mu$ is the dynamic viscosity. The bulk viscosity does not appear explicitly in the boundary condition problem but is relevant for the formation of the steady acoustic streaming flow in the liquid bulk in the absence of

the particle. The velocities in the fluid are:

$$c_\ell(\omega) = c_0\sqrt{1 + \mathrm{i}2\omega\mu/(c_0^2\rho_0)} \approx c_0, \tag{22}$$

$$c_t(\omega) \qquad = (1-\mathrm{i})\sqrt{\omega\mu/(2\rho_0)}, \tag{23}$$

where the latter is related to the shear wave rapidly damped inside the boundary layer of thickness $\delta = (2\mu/\rho\omega)^{1/2}$.

Finally the right hand side vector $\mathbf{B}$ writes:

$$B_1 = -x_\ell j_n'(x_\ell), \tag{24}$$

$$B_2 = -j_n(x_\ell), \tag{25}$$

$$B_3 = -G(b_n j_n(x_\ell) - 4x_\ell j_n'(x_\ell)), \tag{26}$$

$$B_4 = -G(x_\ell j_n'(x_\ell) - j_n(x_\ell)). \tag{27}$$

$R_n$ is the first unknown coefficient of $X$. This system agrees with the original derivation of Epstein and Allegra [8, 9] after correction of sign errors. However, on one hand we made use of the Bessel differential equation to eliminate second order derivatives, on the other, thermal dissipation within the solid particle or host fluid were not considered. For polymers like polystyrene, the main attenuation mechanism does not involve volume changes and therefore minimizing thermal losses. Additionally, the assumption holds for a solid particle of polymer in low heat-conducting fluids such as water where the main attenuation processes arise from viscous dissipation. Note that a comprehensive derivation of this system was recently published [10] where the thermal boundary layers were included. For small particles in the Rayleigh limit, thermal effects are shown to affect the monopolar particle oscillation that is, however, not excited as long as the particle lies on the propagation axis of an AV[5]. Obtaining accurate numerical solutions of this system can be quite difficult. Since the viscosity is small, the parameter $x_t$ can become large and Hankel functions, that grow exponentially in that limit, rapidly reach the accuracy limit in double precision. If this occurs, the matrix $\mathbf{A}$ becomes numerically singular. To reach the required accuracy, we used an arbitrary precision library, Ref. [11].

**Quadrupolar dissipation contributions in the long-wavelength regime**

An unexpected result was the need to include quadrupolar contributions to the total acoustic torque as written in Eqs.(1)-(2). Indeed, it is usually assumed that in the long-wavelength regime ($a/\lambda \ll 1$), monopolar and dipolar vibrations of a spherical object suffice to calculate the strength of the scattered field and thereafter, second order effects as the radiation force and torque. In the case of the force, dissipation amounts to a small correction to the average exchange of the flux of momentum in focused beams (not plane waves). However, in the specific case of the torque, the effect grows as a consequence of dissipation only. Indeed, the terms in Eq.2 can be shown to be largely dominated by the dissipation contributions included in the scattering coefficients $R_n$ calculated in the previous section.

In figure 3, we plot the imaginary and real parts of the complex scattering coefficients. Corrections due to dissipation principally affect the real parts of $R_n$. In the case of a perfect polystyrene particle suspended in viscous water ($\mu = 10^{-3}$ Pa·s), the calculation (plain lines) agrees well with analytical expressions (dash-dotted lines) recently published [12], up to approximatively $a/\lambda \sim 0.08$. However, it is also evident that the magnitude of the quadrupolar mode $\Re(R_2)$ is not negligible and actually largely exceeds the dissipation correction to the dipole. This seems to be particularly important for low density polymers such as polystyrene and PMMA, for which the dipolar strength is maintained low as a consequence of the weak density contrast between the particle and the host fluid. For an absorbing sphere suspended in water considered this time as a perfect fluid, we also retrieve analytical expressions (dash-dotted curve) for the dipole [13], the effect of the quadrupole starts to account in a regime for which the long-wavelength criteria starts to be arguable. It will however very rapidly dominate the torque calculation.

These observations translate directly into Eq.(2) and appear in the torque plots, Fig.2(c) in the main text.

**Far-field approach to calculate the torque**

The torque calculation considered is based on a far-field approach. Indeed, Eqs.1 and 2 are obtained by integrating the radiation stress tensor, or Brillouin stress tensor on a fictitious sphere enclosing the object in the fluid bulk assumed to be perfect. This is possible

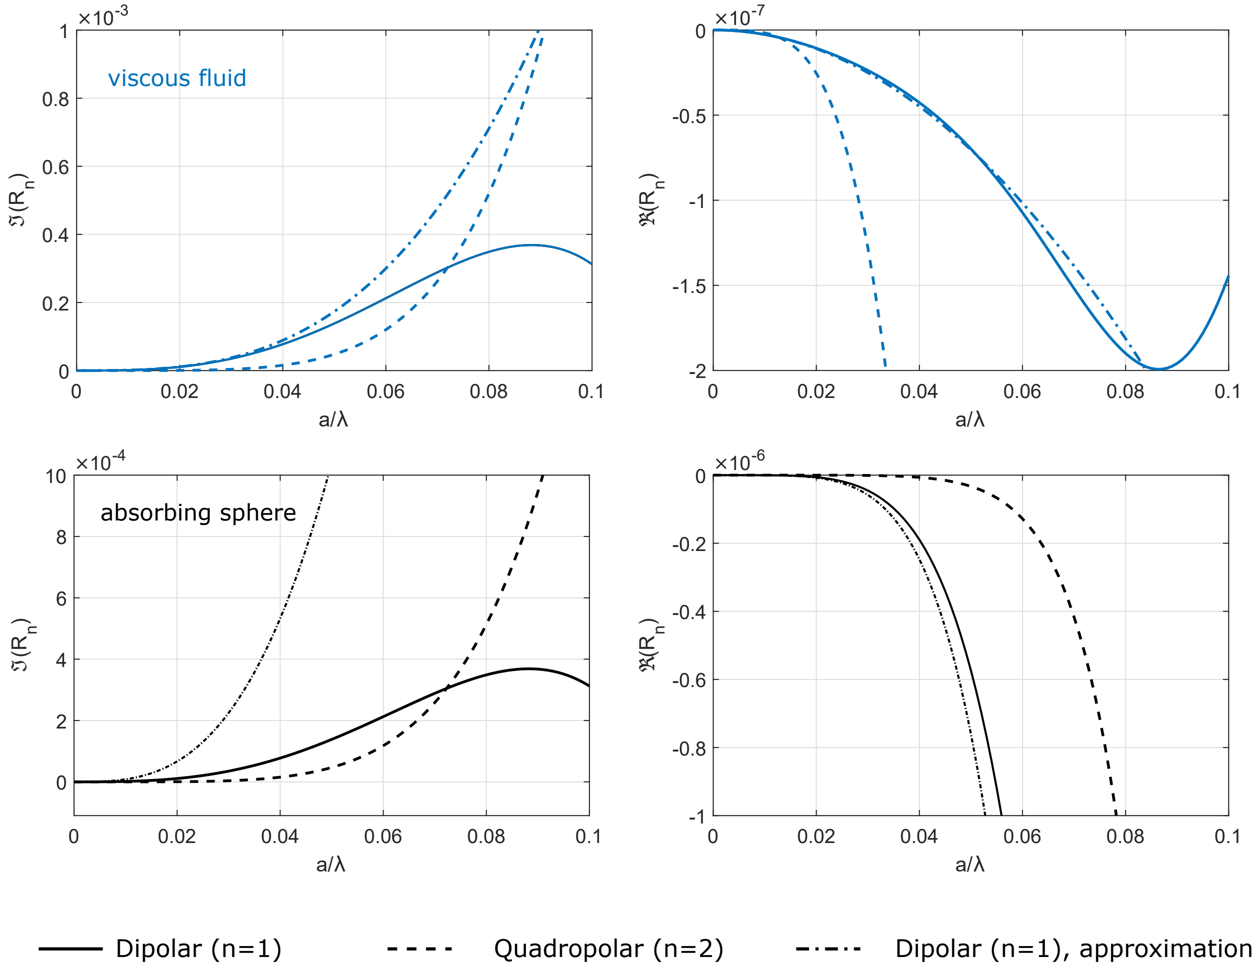


FIG. 3. Dipolar and quadroplar scattering coefficients. In a viscous fluid (Top) for a non-absorbing polystyrene sphere. In a perfect fluid (bottom) for polystyrene sphere allowing for the absorption of shear and longitudinal waves.

as a result of momentum conservation in the bulk in the absence of any body force in the volume in between the object and an arbitrarily surface enclosing the sphere. Such approach was successfully applied to calculate the force acting on a small spherical object [14] and the torque on axisymmetric absorbing objects [2]. Importantly, viscous and absorption processes in, and around, the object are included as corrections to the scattered wave in the far field. An immediate consequence being that it is sufficient to find a solution to the viscous momentum equation to *first order*. However, in the literature, it is also common to solve the average momentum equation up to second order for the velocity field in a viscous fluid to calculate the torque acting on the particle [15–18]. The torque is understood as a consequence of a second order stress and flow, originally analyzed by Schlitling [19], building

up in the vicinity of the sphere. This generated steady second order flow is not confined to the inside of the boundary layer [20] but, however, it can be disregarded in calculating the mean stress tensor far from the sphere inasmuch as it would constitute fourth order corrections. This does not suggest that this inner streaming flow will not exist, but instead, that it is unnecessary to solve the viscous momentum equations in the vicinity of the sphere to second order to calculate the acoustic force or torque. For this reason, the two different approaches are shown to give the exact same result for the torque [21].

---

* Currently at Department of Chemical Engineering, Imperial College London.; d.baresch@imperial.ac.uk

[1] D. Baresch, J.-L. Thomas, and R. Marchiano, J. Acoust. Soc. Am. **133**, 25 (2013).

[2] L. Zhang and P. L. Marston, The Journal of the Acoustical Society of America **129**, 1679 (2011).

[3] L. Zhang and P. L. Marston, Physical Review E - Statistical, Nonlinear, and Soft Matter Physics **84** (2011), 10.1103/PhysRevE.84.065601.

[4] D. Baresch, J.-L. Thomas, and R. Marchiano, J. App. Phys. **113**, 184901 (2013).

[5] D. Baresch, J.-L. Thomas, and R. Marchiano, Phys. Rev. Lett. **116**, 024301 (2016).

[6] Y. Takagi, T. Hosokawa, K. Hoshikawa, H. Kobayashi, and Y. Hiki, Journal of the Physical Society of Japan **76**, 024604 (2007).

[7] R. Kono, Journal of the Physical Society of Japan **15**, 718 (1960).

[8] P. S. Epstein and R. R. Carhart, J. Acoust. Soc. Am. **25**, 553 (1953).

[9] J. R. Allegra and S. A. Hawley, J. Acoust. Soc. Am. **51**, 1545 (1972).

[10] J. T. Karlsen and H. Bruus, Phys. Rev. E **92**, 043010 (2015).

[11] F. Johansson *et al.*, *mpmath: a Python library for arbitrary-precision floating-point arithmetic (version 0.18)* (2013), `http://mpmath.org/`.

[12] P. B. Muller, M. Rossi, A. G. Marín, R. Barnkob, P. Augustsson, T. Laurell, C. J. Kähler, and H. Bruus, Phys. Rev. E **88**, 023006 (2013).

[13] G. T. Silva, The Journal of the Acoustical Society of America **136**, 2405 (2014).

[14] M. Settnes and H. Bruus, Physical Review E **85**, 016327 (2012).

[15] A. Biswas, E. Leung, and E. Trinh, The Journal of the Acoustical Society of America **90**, 1502 (1991).

[16] A. Lamprecht, T. Schwarz, J. Wang, and J. Dual, The Journal of the Acoustical Society of America **138**, 23 (2015).

[17] P. Hahn, A. Lamprecht, and J. Dual, Lab on a Chip **16**, 4581 (2016).

[18] I. Bernard, A. A. Doinikov, P. Marmottant, D. Rabaud, C. Poulain, and P. Thibault, Lab on a Chip **17**, 2470 (2017).

[19] M. Wiklund, R. Green, and M. Ohlin, Lab on a Chip **12**, 2438 (2012).

[20] F. Busse and T. Wang, The Journal of the Acoustical Society of America **69**, 1634 (1981).

[21] L. Zhang and P. L. Marston, The Journal of the Acoustical Society of America **136**, 2917 (2014).
